# Supplementary material for: RaBit: Parametric Modeling of 3D Biped Cartoon Characters with a Topological-consistent Dataset
Source: arXiv:2303.12564 source file (2023-03-24)
Supplement: Supplementary file 1 [file fig_assemble.tex]

\begin{figure}
     \centering
     \begin{subfigure}[b]{0.1\textwidth}
         \centering
         \includegraphics[width=\textwidth]{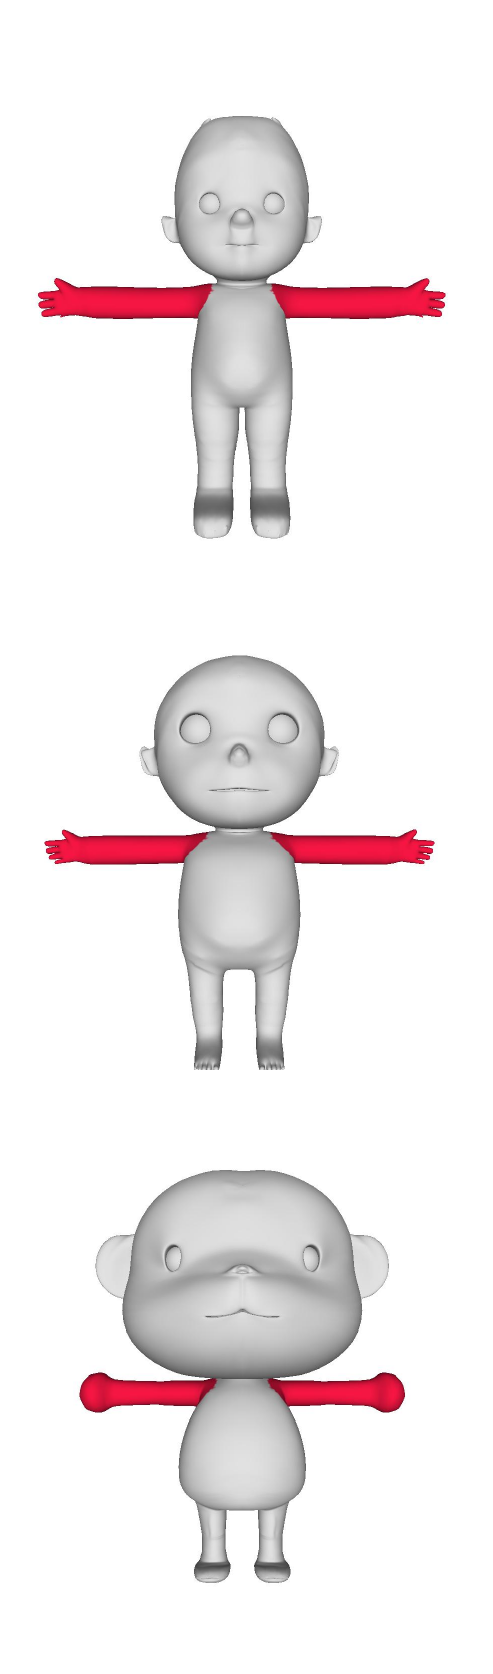}
         \caption{Arms}
     \end{subfigure}
     \hfill\hspace{-4mm}
     \begin{subfigure}[b]{0.1\textwidth}
         \centering
         \includegraphics[width=\textwidth]{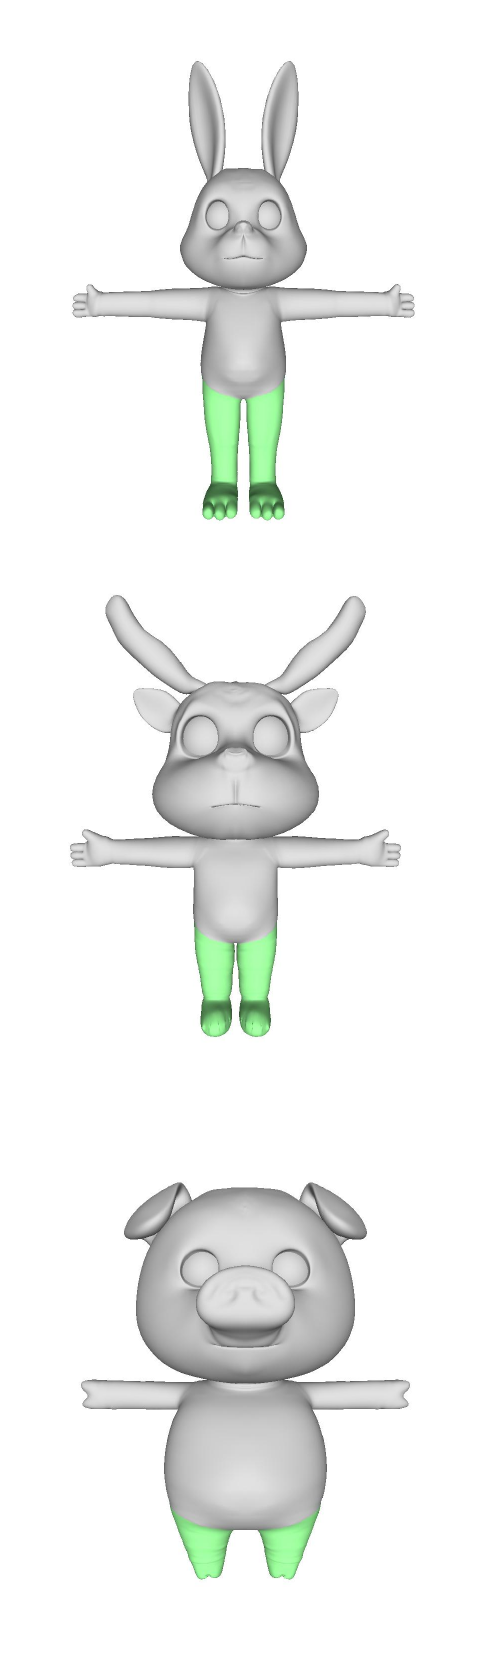}
         \caption{Legs}
     \end{subfigure}
     \hfill\hspace{-4mm}
     \begin{subfigure}[b]{0.1\textwidth}
         \centering
         \includegraphics[width=\textwidth]{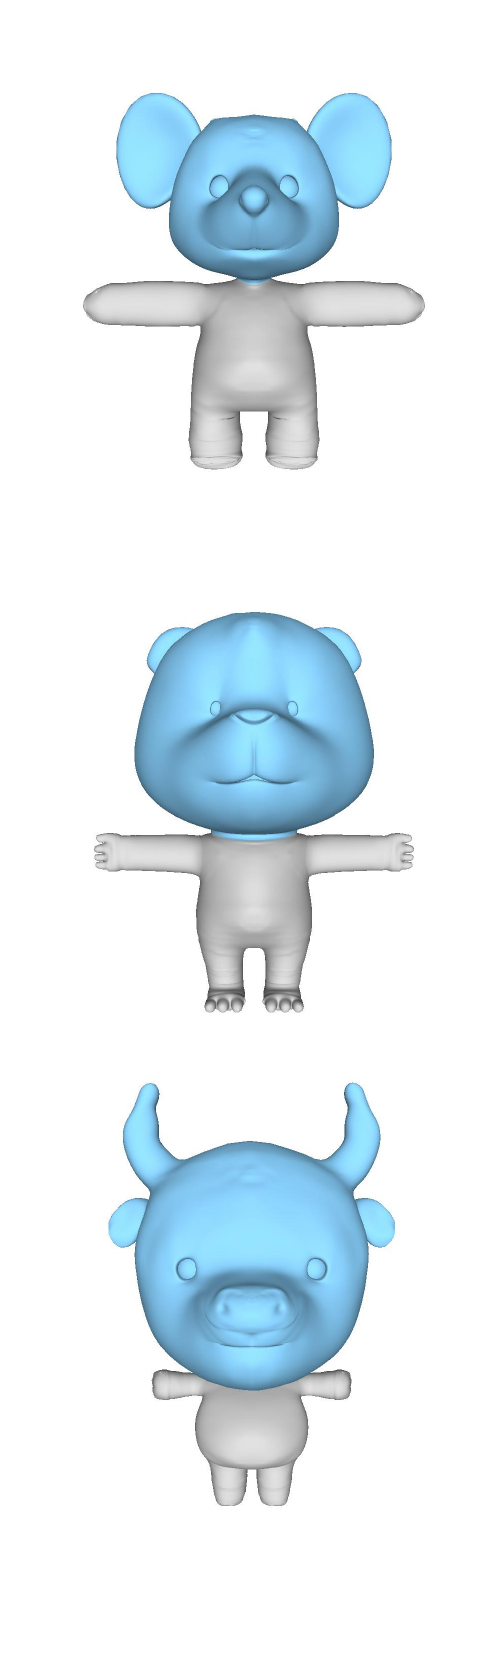}
         \caption{Head}
     \end{subfigure}
     \hfill\hspace{-4mm}
     \begin{subfigure}[b]{0.1\textwidth}
         \centering
         \includegraphics[width=\textwidth]{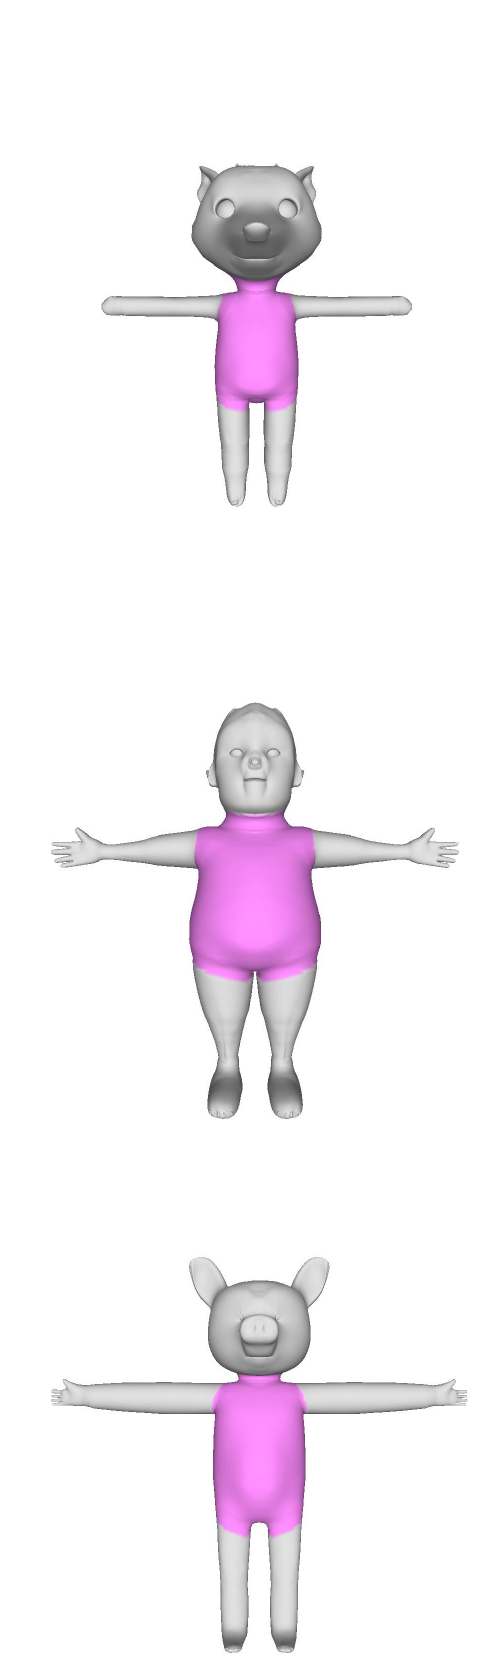}
         \caption{Body}
     \end{subfigure}
     \hfill\hspace{-4mm}
     \begin{subfigure}[b]{0.1\textwidth}
         \centering
         \includegraphics[width=\textwidth]{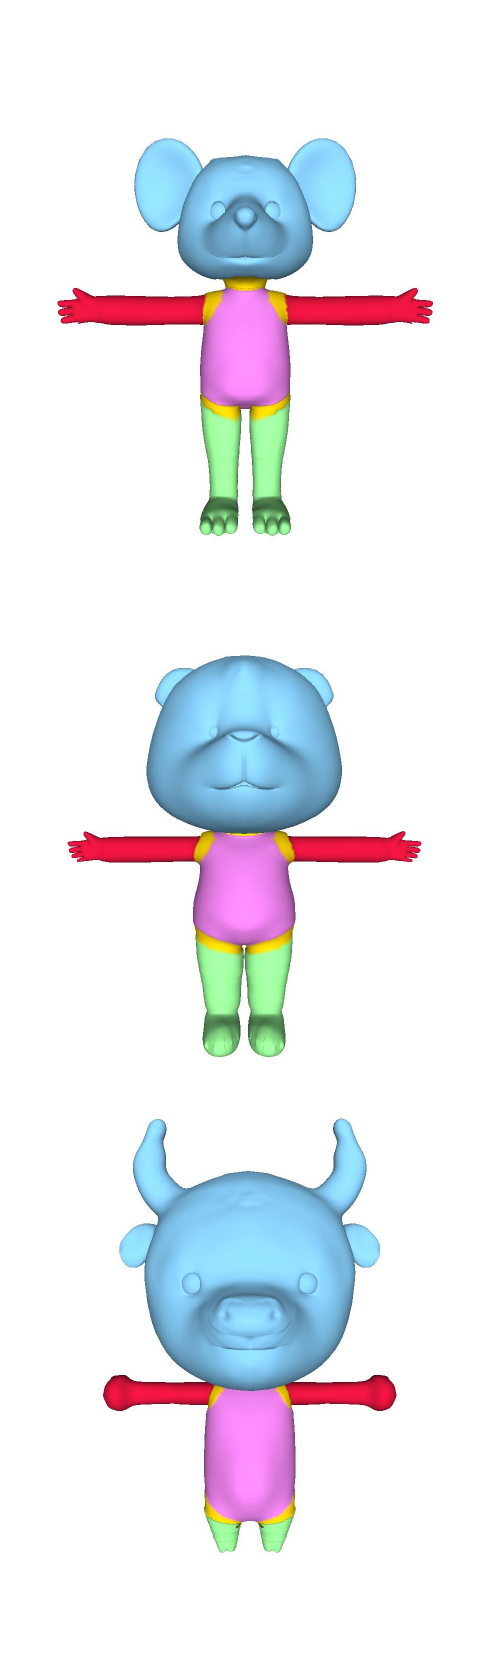}
         \caption{Concat}
     \end{subfigure}
     \caption{\textbf{Part-aware Sample}. By concating embeddings representing differet parts from different model, we can sample a new model(e) which assemble parts (a-d) from different models. In column (e), yellow texture means the collision between two different parts.}
\end{figure}
